# Supplementary material for: Extreme Value Monte Carlo Tree Search for Classical Planning
Source: arXiv:2405.18248 source file (2026-03-26)
Supplement: Supplementary file 1 [file supplemental.pdf]

# Appendix

## S1. Domain-Independent Heuristics in Classical Planning

A domain-independent heuristic function $h$ in classical planning is a function of a state $s$ and the problem $[P, A, I, G]$, but the notation $h(s)$ usually omits the latter. In addition to what we discussed in the main article, this section also uses a notation $h(s, G)$. It returns an estimate of the cumulative cost from $s$ to one of the goal states (states that satisfy $G$), typically through a symbolic, non-statistical means including problem relaxation and abstraction. Notable state-of-the-art functions that appear in this paper includes $h^{\text{FF}}, h^{\max}, h^{\text{add}}, h^{\text{GC}}$ (Hoffmann & Nebel, 2001; Bonet & Geffner, 2001; Fikes et al., 1972).

A significant class of heuristics is called delete relaxation heuristics, which solve a relaxed problem which does not contain delete effects, and then returns the cost of the solution of the relaxed problem as an output. The cost of the optimal solution of a delete relaxed planning problem from a state $s$ is denoted by $h^+(s)$, but this is too expensive to compute in practice (NP-complete) (Bylander, 1996). Therefore, practical heuristics typically try to obtain its further relaxations that can be computed in polynomial time.

One such admissible heuristic based on delete-relaxation is called $h^{\max}$ (Bonet & Geffner, 2001) that is recursively defined as follows:

$$h^{\max}(s, G) = \max_{p \in G} \begin{cases} 0 \text{ if } p \in s. \text{ Otherwise,} \\ \min_{\{a \in A | p \in \text{ADD}(a)\}} \\ \quad \left[\text{C}(a) + h^{\text{add}}(s, \text{PRE}(a))\right]. \end{cases} \tag{1}$$

Its inadmissible variant is called additive heuristics $h^{\text{add}}$ (Bonet & Geffner, 2001) that is recursively defined as follows:

$$h^{\text{add}}(s, G) = \sum_{p \in G} \begin{cases} 0 \text{ if } p \in s. \text{ Otherwise,} \\ \min_{\{a \in A | p \in \text{ADD}(a)\}} \\ \quad \left[\text{C}(a) + h^{\text{add}}(s, \text{PRE}(a))\right]. \end{cases} \tag{2}$$

Another inadmissible delete-relaxation heuristics called $h^{\text{FF}}$ (Hoffmann & Nebel, 2001) is defined based on another heuristics $h$, such as $h = h^{\text{add}}$, as a subprocedure. For each unachieved subgoal $p \in G \setminus s$, the action $a$ that adds $p$ with the minimal $[\text{C}(a) + h(s, \text{PRE}(a))]$ is conceptually "the cheapest action that achieves a subgoal $p$ for the first time under delete relaxation", called the *cheapest achiever / best supporter* $\text{bs}(p, s, h)$ of $p$. $h^{\text{FF}}$ is defined as the sum of actions in a relaxed plan $\Pi^+$ constructed as follows:

$$h^{\text{FF}}(s, G, h) = \sum_{a \in \Pi^+(s,G,h)} \text{C}(a) \tag{3}$$

$$\Pi^+(s, G, h) = \bigcup_{p \in G} \begin{cases} \emptyset \text{ if } p \in s. \text{ Otherwise,} \\ \{a\} \cup \Pi^+(s, \text{PRE}(a)) \\ \quad \text{where } a = \text{bs}(p, s, h). \end{cases} \tag{4}$$

$$\text{bs}(p, s, h) = \operatorname*{arg\,min}_{\{a \in A | p \in \text{ADD}(a)\}} \left[\text{C}(a) + h(s, \text{PRE}(a))\right]. \tag{5}$$

Goal Count heuristics $h^{\text{GC}}$ is a simple heuristic proposed in (Fikes et al., 1972) that counts the number of propositions that are not satisfied yet. $[\text{condition}]$ is a cronecker's delta / indicator function that returns 1 when the condition is satisfied.

$$h^{\text{GC}}(s, G) = \sum_{p \in G} [\![p \notin s]\!]. \tag{6}$$

## S2. Detailed Explanation for the Base MCTS for Graph Search

Alg. 1 shows the pseudocode of MCTS adjusted for graph search (Schulte & Keller, 2014). Aside from what was described from the main section, it has a node-locking mechanism that avoids duplicate search effort.

Following THTS, our MCTS has a hash table that implements a *CLOSE* list and a *Transposition Table* (TT). A CLOSE list stores the generated states and avoids instantiating nodes with duplicate states. A TT stores various information about the states such as the parent information and the action used at the parent. The close list is implemented by a lock mechanism.

Since an efficient graph search algorithm must avoid visiting the same state multiple times, MCTS for graph search marks certain nodes as *locked*, and excludes them from the selection candidates. A node is locked either (1) when a node is a dead-end that will never reach a goal (detected by having no applicable actions, by a heuristic function, or other facilities), (2) when there is a node with the same state in the search tree with a smaller g-value, (3) when all of its children are locked, or (4) when a node is a goal (relevant in an anytime iterated search setting (Richter et al., 2010; 2011), but not in this paper). Thus, in the expansion step, when a generated node $n$ has the same state as a node $n'$ already in the search tree, MCTS discards $n$ if $g(n) > g(n')$, else moves the subtree of $n'$ to $n$ and marks $n'$ as locked. It also implicitly detects a cycle, as this is identical to the duplicate detection in Dijkstra/A*/GBFS.

The queueing step backpropagates necessary information from the leaf to the root. Efficient backpropagation uses a priority queue ordered by descending $g$-value. The queue is initialized with the expanded node $p$; each newly generated node $n$ that is not discarded is inserted into the queue, and if a node $n'$ for the same state was already present in the tree it is also inserted into the queue. In each backpropagation iteration, (1) the enqueued node with the highest $g$-value is popped, (2) its information is updated by aggregating its children's information (including the lock status), (3) and its parent is queued.

## S3. Proof of MLE

We show the maximum likelihood estimate of Gaussian, Power, and Uniform distribution Thm. 1-6. First, let us restate the definition of MLE:

**Definition 1.** *Given i.i.d. samples $x_1, \ldots, x_N \sim p(\mathrm{x}|\theta)$, the Maximum Likelihood Estimate (MLE) of the parameter $\theta$ is:*

$$\begin{aligned}\hat{\theta} &= \arg\max_{\theta} p(x_1, \ldots, x_N|\theta) \\ &= \arg\max_{\theta} \log p(x_1, \ldots, x_N|\theta).\end{aligned}$$

Sometimes the MLE is solved by the following equation for the target parameter $\theta$.

$$\begin{aligned}0 &= \frac{\partial}{\partial\theta} p(x_1, \ldots, x_N|\theta) \\ &= \frac{\partial}{\partial\theta} \log p(x_1, \ldots, x_N|\theta) \\ &= \frac{\partial}{\partial\theta} \log \prod_i p(x_i|\theta) = \frac{\partial}{\partial\theta} \sum_i \log p(x_i|\theta).\end{aligned}$$

An estimator that is obtained by maximizing some quantity is called an *M-estimator*. MLE is an M-estimator. Some M-estimators can be solved by setting the derivatives to zero, in which case they are called *Z-estimator*. Not all M-estimators are solved in this way, as seen below ($l$ and $u$ of Power and Uniform).

**Theorem 1.** *Given i.i.d. $x_1, \ldots, x_N \sim \mathcal{N}(\mathrm{x}|\mu, \sigma)$, the Maximum Likelihood Estimate of $\mu$ is the sample average $\hat{\mu} = \frac{1}{N}\sum_i x_i$. Similarly, the Maximum Likelihood Estimate of $\sigma^2$ is the sample variance $\frac{1}{N-1}\sum_i (x_i - \hat{\mu})$.*

*Proof.* For $\mu$,

$$\begin{aligned}0 &= \frac{\partial}{\partial\mu} \sum_i \log \mathcal{N}(x_i|\mu, \sigma) \\ &= \frac{\partial}{\partial\mu} \sum_i \log \left( \frac{1}{\sqrt{2\pi\sigma^2}} \exp - \frac{(x_i - \mu)^2}{2\sigma^2} \right) \\ &= \frac{\partial}{\partial\mu} \sum_i \left( - \frac{(x_i - \mu)^2}{2\sigma^2} - \log\sqrt{2\pi\sigma^2} \right) \\ &= \frac{\partial}{\partial\mu} \sum_i \left( \frac{-x_i^2 + 2\mu x_i - \mu^2}{2\sigma^2} - \log\sqrt{2\pi\sigma^2} \right) \\ &= \sum_i \frac{2x_i - 2\mu}{2\sigma^2}. \quad \therefore \hat{\mu} = \frac{\sum_i x_i}{N}.\end{aligned}$$

For $\sigma^2$,

$$\begin{aligned}0 &= \frac{\partial}{\partial\sigma^2} \sum_i \log \mathcal{N}(x_i|\mu, \sigma) \\ &= \frac{\partial}{\partial\sigma^2} \sum_i \log \left( \frac{1}{\sqrt{2\pi\sigma^2}} \exp - \frac{(x_i - \mu)^2}{2\sigma^2} \right) \\ &= \frac{\partial}{\partial\sigma^2} \sum_i \left( - \frac{(x_i - \mu)^2}{2\sigma^2} - \frac{\log 2\pi + \log\sigma^2}{2} \right) \\ &= \sum_i \left( \frac{(x_i - \mu)^2}{2(\sigma^2)^2} - \frac{1}{2\sigma^2} \right). \\ \therefore \hat{\sigma}^2 &= \frac{\sum_i (x_i - \mu)^2}{N} = \frac{\sum_i (x_i - \hat{\mu})^2}{N - 1}.\end{aligned}$$

□

**Theorem 2.** *Given i.i.d. $x_1, \ldots, x_N \sim \mathrm{Pow}(\mathrm{x}|u, a)$, $\hat{u} = \max_i x_i$ and $\hat{a} = \left(\log\hat{u} - \frac{1}{N}\sum_i \log x_i\right)^{-1}$.*

*Proof.* For $u$, we cannot use the differentiation-based proof. Instead, we maximize the log likelihood directly.

$$\begin{aligned}&\sum_i \log \mathrm{Pow}(x_i|u, a) \\ &= \sum_i \log \frac{a x_i^{a-1}}{u^a} \\ &= \sum_i (\log a + (a-1)\log x_i - a\log u).\end{aligned}$$

The value of $u$ that maximizes this formula is the infimum of possible values $u$ can take. Since $\forall i; x_i \leq u$, $u = \max_i x_i$.

For $a$,

$$\begin{aligned}0 &= \frac{\partial}{\partial a} \sum_i \log \mathrm{Pow}(x_i|u, a) \\ &= \frac{\partial}{\partial a} \sum_i \log \frac{a x_i^{a-1}}{u^a} \\ &= \frac{\partial}{\partial a} \sum_i (\log a + (a-1)\log x_i - a\log u) \\ &= \sum_i (\frac{1}{a} + \log x_i - \log u). \\ \therefore a &= \left(\log u - \tfrac{1}{N}\textstyle\sum_i \log x_i\right)^{-1}.\end{aligned}$$

□

**Theorem 3.** *Given i.i.d.* $x_1, \ldots, x_N \sim U(\mathrm{x}|l, u)$*,* $\hat{u} = \max_i x_i$ *and* $\hat{l} = \min_i x_i$.

*Proof.* For $u$, we cannot use the differentiation-based proof. Instead, we maximize the log likelihood directly.

$$\begin{aligned} &\sum_i \log U(x_i|l, u) \\ &= \sum_i \log \frac{1}{u - l} \\ &= \sum_i - \log(u - l). \end{aligned}$$

The value of $u$ that maximizes this formula is the infimum of possible values $u$ can take. Since $\forall i; x_i \leq u$, $u = \max_i x_i$.

Similarly, the value of $l$ that maximizes this formula is the supremum of possible values $l$ can take. Since $\forall i; l \leq x_i$, $l = \min_i x_i$. □

**Algorithm 1** High-level general MCTS. **Input**: Root node $r$, successor function $S$, NEC $f$, heuristic function $h$, priority queue $Q$ sorted by $g$. Initialize $\forall n; g(n) \leftarrow \infty$.

```
while True do
  Parent p ← r
  while not leaf p do      # Selection
    p ← arg min_{n∈S(p)} f(n)
  Q ← {p}
  for n ∈ S(p) do      # Expansion
    return n if n is goal.      # Early goal detection
    if ∃n′ already in tree with same state s_{n′} = s_n then
      if g(n) > g(n′) then
        continue
      Lock n′, S(n) ← S(n′), Q ← Q ∪ {n, n′}
    else
      Compute h(s_n)      # Evaluation
      Q ← Q ∪ {n}
  while n ← Q.POPMAX() do      # Backpropagation
    Update n's statistics and lock status
    Q ← Q ∪ {n's parent}
```

## S4. Proof of Bandit Algorithms

To help understand the proof of various confidence bounds, we first describe the general procedure for proving the regret of bandit algorithms, demonstrate the proof of UCB1 using this scheme, then finally show the proof of other bandits.

The ingredients for proving an upper/lower confidence bound are as follows:

- **Ingredient 1: The main term and the exploration term.** For example, in the standard UCB1 (Auer et al., 2002), the *main term* is the empirical mean $\hat{\mu}$ while the *exploration term* is $c\sqrt{\frac{2\log T}{n_i}}$. Their forms are heavily affected by the proof of the upper bound on the regret, therefore it is not like you can use an arbitrary exploration term you came up with.
- **Ingredient 2: A specification of reward distributions.** For example, in the standard UCB1 (Auer et al., 2002), one assumes a reward distribution bounded in $[0, b]$. Different algorithms assume different reward distributions, and in general, more information about the distribution gives a tighter bound (and faster convergence). For example, one can assume an unbounded distribution with known variance, etc.
- **Ingredient 3: A concentration inequality.** It is also called a tail probability bound. For example, in the standard UCB1, one uses Hoeffding's inequality. Different algorithms use different inequalities to prove the bound, based on what reward distribution it assumes and what main term it uses. Examples include the Chernoff bound, Chebishev's inequality, Bernstein's inequality, Bennett's inequality, etc. Note that the inequality may be two-sided or one-sided.

The general procedure for proving the bound is as follows.

1. Let the main term be a random variable $\mathrm{X}_n$ and the exploration term be $\delta$. Then write down the concentration inequality for $\mathrm{X}_n$ as follows.
   - $P(|\mathrm{X}_n - \mathbb{E}[\mathrm{X}_n]| \geq \delta) \leq F(\delta)$. (two-sided)

   $F$ is an inequality-specific formula. If necessary, simplify the inequality based on the assumptions made in the reward distribution, e.g., bounds, mean, variance.
2. Expand $|\mathrm{X}_n - \mathbb{E}[\mathrm{X}_n]| \geq \delta$ into $\delta \geq \mathrm{X}_n - \mathbb{E}[\mathrm{X}_n] \geq -\delta$.
3. Change the notations to model the bandit problem because each concentration inequality is a general statement about RVs. Before this step, the notation was:
   - $n$ (number of samples)
   - $\mathrm{X}_n$ is a function of i.i.d. random variables $(\mathrm{x}_1, \ldots, \mathrm{x}_n)$
   - $\mathbb{E}[\mathrm{X}_n] = \mathbb{E}[\mathrm{x}_1] = \ldots = \mathbb{E}[\mathrm{x}_n]$ is assumed.

   For example,
   - $\mu_n = \frac{1}{n}\sum_{i=1}^{n} \mathrm{x}_i$
   - $\mathbb{E}[\mu_n] = \mathbb{E}[\mathrm{x}_1] = \ldots = \mathbb{E}[\mathrm{x}_n]$

   After the change, they correspond to:
   - $n_i$ (number of pulls of arm $i$).
   - $\hat{X}_i$ (empirical value of arm $i$ from $n_i$ pulls),
   - $X_i$ (true value of arm $i$).

   For example,
   - $\hat{\mu}_i$ (sample mean of arm $i$ from $n_i$ pulls),
   - $\mu_i$ (true mean of arm $i$),
4. Let $i$ be a suboptimal arm, $*$ be an optimal arm, $\mathrm{UCB}_i = \hat{\mu}_i + \delta$, and $\mathrm{LCB}_i = \hat{\mu}_i - \delta$. Derive the relationship between $\delta$ and the gap $\Delta_i = \mu_i - \mu_*$ so that the following conditions for the best arm holds:
   - $\mathrm{UCB}_i \leq \mathrm{UCB}_*$ (for maximization)
   - $\mathrm{LCB}_i \geq \mathrm{LCB}_*$ (for minimization)

   This results in $2\delta \leq \Delta_i$.
5. Replace the $\delta$ with the exploration term. For example, in UCB1, $\delta = \sqrt{\frac{2\log T}{n_i}}$.
6. Derive the lower bound $L$ for $n_i$ from $2\delta \leq \Delta_i$.
7. Find the upper-bound of the probability of selecting a sub-optimal arm $i$. This is typically done by a union-bound argument.
8. Derive the upper bound of the expected number of pulls $\mathbb{E}[n_i]$ of a suboptimal arm $i$ using a triple loop summation. This is typically the heaviest part that needs mathematical tricks. The tricks do not seem generally transferable between approaches.
9. Finally, derive an upper bound of the regret $TX_* - \sum_{i=1}^{K} X_i \mathbb{E}[n_i]$ by

$$TX_* - \sum_{i=1}^{K} X_i \mathbb{E}[n_i] = \sum_{i=1}^{K} (X_* - X_i)\mathbb{E}[n_i] = \sum_{i=1}^{K} \Delta_i \mathbb{E}[n_i].$$

## S5. The Proof of UCB1

Now we prove the logarithmic upper bound of the cumulative regret of the UCB1 $\hat{\mu}_i - c\sqrt{\frac{2\log T}{n_i}}$ where $\hat{\mu}_i$ is the empirical mean of samples from arm $i$, $n_i$ is the number of pulls from arm $i$, and $T = \sum_{i=1}^{K} n_i$ is the total pulls from all $K$ arms.

1. UCB1 assumes a reward distribution with a known bound. For such a distribution, we can use Hoeffding's inequality. Given RVs $\mathrm{x}_1 \ldots \mathrm{x}_n$, where $\mathrm{x}_i \in [l_i, u_i]$, and their sum $\mathrm{S}_n = \sum_{i=1}^{n} \mathrm{x}_i$,

$$P(|\mathrm{S}_n - \mathbb{E}[\mathrm{S}_n]| \geq \epsilon) \leq 2\exp - \frac{2\epsilon^2}{\sum_{i=1}^{n}(u_i - l_i)^2}.$$

Using $\delta = \frac{\epsilon}{n}$ and $\mu_n = \frac{\mathrm{S}_n}{n}$,

$$P(|\mu_n - \mathbb{E}[\mu_n] \geq \delta|) \leq 2\exp - \frac{2n^2\delta^2}{\sum_{i=1}^{n}(u_i - l_i)^2}.$$

UCB1 assumes $\mathrm{x}_i$ are i.i.d. copies, thus $\forall i; u_i - l_i = c$.

$$P(|\mu_n - \mathbb{E}[\mu_n] \geq \delta|) \leq 2\exp - \frac{2n^2\delta^2}{nc^2} = 2\exp - \frac{2n\delta^2}{c^2}.$$

2. Expanding the two-sided error:

$$\delta \geq \mu_n - \mathbb{E}[\mu_n] \geq -\delta.$$

3. Changing the notation:

$$\delta \geq \hat{\mu}_i - \mu_i \geq -\delta.$$

4. Adding $\mu_i - \delta$ to both sides,

$$\mu_i \geq \hat{\mu}_i - \delta = \mathrm{LCB}_i(T, n_i) \geq \mu_i - 2\delta.$$

Substituting $i = *$ (optimal arm), the first inequality is

$$\mu_* \geq \hat{\mu}_* - \delta = \mathrm{LCB}_*(T, n_*).$$

**Assuming** $2\delta \leq \Delta_i = \mu_i - \mu_*$, the second inequality is

$$\mathrm{LCB}_i(T, n_i) \geq \mu_i - 2\delta \geq \mu_i - \Delta_i = \mu_*.$$

Therefore

$$\mathrm{LCB}_i(T, n_i) \geq \mu_* \geq \mathrm{LCB}_*(T, n_*).$$

5. Let $\delta = c\sqrt{\frac{2\log T}{n_i}}$. Then

$$P(\mu_{n_i} - \mathbb{E}[\mu_{n_i}] \geq \delta) \leq \exp - \frac{2n_i c^2 \frac{2\log T}{n_i}}{c^2} = T^{-4}.$$

6. From $2\delta \leq \Delta_i$, considering $n_i$ is an integer,

$$2c\sqrt{\frac{2\log T}{n_i}} \leq \Delta_i \Leftrightarrow 4c^2\frac{2\log T}{n_i} \leq \Delta_i^2$$
$$\Leftrightarrow \frac{8c^2\log T}{\Delta_i^2} \leq \left\lceil \frac{8c^2\log T}{\Delta_i^2} \right\rceil = L \leq n_i.$$

7. $\mathrm{LCB}_i(T, n_i) \geq \mu_* \geq \mathrm{LCB}_*(T, n_*)$ does not hold when either inequality does not hold. $\mathrm{LCB}_i(T, n_i) \geq \mu_*$ does not hold with probability less than $T^{-4}$. $\mu_* \geq \mathrm{LCB}_i(T, n_*)$ does not hold with probability less than $T^{-4}$. Thus, by union-bound (probability of disjunctions),

$$P(\mathrm{LCB}_i(T, n_i) \leq \mathrm{LCB}_*(T, n_*)) \leq 2T^{-4}.$$

8. Assume we followed the UCB1 strategy, i.e., we pulled the arm that minimizes the LCB. The expected number of pulls $\mathbb{E}[n_i]$ from a suboptimal arm $i$ is as follows. Note that for $K$ arms, every arm is at least pulled once.

$$\begin{aligned}
\mathbb{E}[n_i] &= 1 + \sum_{t=K+1}^{T} P(i \text{ is pulled at time } t) \\
&\leq L + \sum_{t=K+1}^{T} P(i \text{ is pulled at time } t \wedge n_i > L) \\
&= L + \sum_{t=K+1}^{T} P(\forall j; \mathrm{LCB}_j(t, n_j) \geq \mathrm{LCB}_i(t, n_i)) \\
&\leq L + \sum_{t=K+1}^{T} P(\mathrm{LCB}_*(t, n_*) \geq \mathrm{LCB}_i(t, n_i)) \\
&\leq L + \sum_{t=K+1}^{T} P(\exists u, v; \mathrm{LCB}_*(t, u) \geq \mathrm{LCB}_i(t, v)) \\
&\leq L + \sum_{t=K+1}^{T}\sum_{u=1}^{t-1}\sum_{v=L}^{t-1} P(\mathrm{LCB}_*(t, u) \geq \mathrm{LCB}_i(t, v)) \\
&\leq L + \sum_{t=K+1}^{T}\sum_{u=1}^{t-1}\sum_{v=L}^{t-1} 2t^{-4} \\
&\leq L + \sum_{t=1}^{\infty}\sum_{u=1}^{t}\sum_{v=1}^{t} 2t^{-4} = L + \sum_{t=1}^{\infty} t^2 \cdot 2t^{-4} \\
&= L + 2\sum_{t=1}^{\infty} t^{-2} = L + 2 \cdot \frac{\pi}{6} = L + \frac{\pi}{3} \\
&\leq c^2\frac{8\log T}{\Delta_i^2} + 1 + \frac{\pi}{3} \quad \because \lceil x \rceil \leq x + 1
\end{aligned}$$

9. The regret is

$$T\mu_* - \sum_{i=1}^{K} \mu_i \mathbb{E}[n_i] = \sum_{i=1}^{K} (\mu_* - \mu_i)\mathbb{E}[n_i] = \sum_{i=1}^{K} \Delta_i \mathbb{E}[n_i]$$

$$\leq \sum_{i=1}^{K} \Delta_i \left( c^2 \frac{8 \log T}{\Delta_i^2} + 1 + \frac{\pi}{3} \right)$$

$$\leq \sum_{i=1}^{K} \left( c^2 \frac{8 \log T}{\Delta_i} + \left(1 + \frac{\pi}{3}\right) \Delta_i \right).$$

## S6. Preliminary for the Proof of UCB1-Normal2

Our analysis begins with a definition of Sub-Gaussian distributions.

**Definition 2.** *(Vershynin, 2018, Proposition 2.5.2, (iv)) A distribution $p(x)$ is* sub-Gaussian *when*

$$\exists t > 0; \mathbb{E}[\exp x^2/t^2] < 2.$$

**Theorem 4.** *A Gaussian distribution with 0-mean $\mathcal{N}(0, \sigma^2)$ (without loss of generality) is sub-Gaussian.*

*Proof.*

$$p(x) = \mathcal{N}(0, \sigma^2) = \frac{1}{\sqrt{2\pi\sigma^2}} \exp -\frac{x^2}{2\sigma^2}.$$

$$\begin{aligned}
\mathbb{E}[\exp x^2/t^2] &= \int_{\mathbb{R}} \exp \frac{x^2}{t^2} \frac{1}{\sqrt{2\pi\sigma^2}} \exp -\frac{x^2}{2\sigma^2} dx \\
&= \frac{1}{\sqrt{2\pi\sigma^2}} \int_{\mathbb{R}} \exp -x^2 \left( \frac{1}{2\sigma^2} - \frac{1}{t^2} \right) dx \\
&= \frac{1}{\sqrt{2\pi\sigma^2}} \int_{\mathbb{R}} \exp -\frac{x^2}{C^2} dx \\
&= \frac{1}{\sqrt{2\pi\sigma^2}} \int_{\mathbb{R}} \exp -y^2 C dy \quad \left( \frac{x}{C} = y \Leftrightarrow dx = C dy \right) \\
&= \frac{C}{\sqrt{2\pi\sigma^2}} \sqrt{\pi} \\
&= \frac{C}{\sqrt{2\sigma^2}}.
\end{aligned}$$

Where

$$\begin{aligned}
\frac{1}{C^2} &= \frac{1}{2\sigma^2} - \frac{1}{t^2} \\
\Leftrightarrow C^2 &= \frac{2\sigma^2 t^2}{t^2 - 2\sigma^2}.
\end{aligned}$$

To show $\mathbb{E}[\exp x^2/t^2] < 2$,

$$\begin{aligned}
\mathbb{E}[\exp x^2/t^2] = \frac{C}{\sqrt{2\sigma^2}} &= \sqrt{\frac{t^2}{t^2 - 2\sigma^2}} < 2, \\
&\Leftrightarrow t^2 < 4(t^2 - 2\sigma^2), \\
&\Leftrightarrow \frac{8}{3}\sigma^2 < t^2.
\end{aligned}$$

□

**Definition 3.** *For a sub-Gaussian RV $x$,*

$$||x|| = \inf \left\{ t > 0 \mid \mathbb{E}[\exp x^2/t^2] < 2 \right\}.$$

**Corollary 1.** *For $p(x) = \mathcal{N}(0, \sigma^2)$, $||x|| = \sqrt{\frac{8}{3}}\sigma$.*

Next, we review the general Hoeffding's inequality for sub-Gaussian distributions ().

**Theorem 5.** *For independent sub-Gaussian RVs $x_1, \ldots, x_n$, let their sum be $S_n = \sum_{i=1}^n x_i$. Then, for any $\delta > 0$,*

$$\begin{aligned}
\Pr(|S_n - \mathbb{E}[S_n]| \leq \delta) &\geq 2 \exp -\frac{\delta^2}{\sum_{i=1}^n ||x_i||^2}, \\
\Pr(S_n - \mathbb{E}[S_n] \leq \delta) &\geq \exp -\frac{\delta^2}{\sum_{i=1}^n ||x_i||^2}, \\
\Pr(\mathbb{E}[S_n] - S_n \leq \delta) &\geq \exp -\frac{\delta^2}{\sum_{i=1}^n ||x_i||^2}.
\end{aligned}$$

*(Two-sided bounds and one-sided upper/lower bounds, respectively.)*

## S7. The Proof of UCB1-Normal2

1. Same as UCB1.

2. According to Hoeffding's inequality for sub-Gaussian RVs $X_1 \dots X_n$ and their sum $S_n = \sum_{i=1}^n X_i$,

$$P(S_n - \mathbb{E}[S_n] \geq \epsilon) \leq \exp - \frac{\epsilon^2}{\sum_{i=1}^n ||X_i||^2}.$$

3. Using $\delta = \frac{\epsilon}{n}$,

$$P(\mu_n - \mathbb{E}[\mu_n] \geq \delta) \leq \exp - \frac{n^2\delta^2}{\sum_{i=1}^n ||X_i||^2}.$$

4. We assume $X_i = \mathcal{N}(\mu, \sigma^2)$, thus $||X_i||^2 = \frac{8}{3}\sigma^2$.

$$P(\mu_n - \mathbb{E}[\mu_n] \geq \delta) \leq \exp - \frac{3n^2\delta^2}{8n\sigma^2} = \exp - \frac{3n\delta^2}{8\sigma^2}.$$

5. Same as UCB1.

6. Same as UCB1.

7. Same as UCB1.

8. Let $\delta = \hat{\sigma}\sqrt{\log T}$. Then

$$P(A : \mu_{n_i} - \mathbb{E}[\mu_{n_i}] \geq \delta) \leq \exp - \frac{3n_i\hat{\sigma}^2 \log T}{8\sigma^2} = T^{-\frac{3n_i\hat{\sigma}^2}{8\sigma^2}}.$$

The trick starts here. The formula above is problematic because we do not know the true variance $\sigma^2$. However, if event $B : \frac{n_i\hat{\sigma}^2}{\sigma^2} \geq X$ holds for some $X > 0$, we have

$$T^{-\frac{3n_i\hat{\sigma}^2}{8\sigma^2}} \leq T^{-\frac{3}{8}X}.$$

One issue with this approach is that the two events $A, B$ may be correlated. To address the issue, we further upper-bound the probability by union-bound. Let $P(B) = \alpha$ which is close to 1. Then

$$\begin{aligned} P(\neg(A \wedge B)) = P(\neg A \vee \neg B) &\leq P(\neg A) + P(\neg B). \\ 1 - P(A \wedge B) &\leq 1 - P(A) + P(\neg B). \\ P(A) &\leq P(A \wedge B) + P(\neg B). \\ \therefore P(\mu_{n_i} - \mathbb{E}[\mu_{n_i}] \geq \delta) &\leq T^{-\frac{3}{8}X} + 1 - \alpha. \end{aligned}$$

We next obtain $X$ that satisfies $P(B) = \alpha$. We use the fact that $\frac{n_i\hat{\sigma}^2}{\sigma^2}$ follows a Chi-Squared distribution $\chi^2(n_i)$ with a degree of freedom $n_i$. Then $X = \chi^2_{1-\alpha,n_i}$, the upper-tail critical value of $\chi^2$ distribution with degree of freedom $n_i$ and significance level $\alpha$, because

$$\begin{aligned} P(\neg B) &= P(\frac{n_i\hat{\sigma}^2}{\sigma^2} < \chi^2_{1-\alpha,n_i}) \\ &= \chi^2(\frac{n_i\hat{\sigma}^2}{\sigma^2} < \chi^2_{1-\alpha,n_i} \mid n_i) = 1 - \alpha. \end{aligned}$$

9. From $2\delta \leq \Delta_i$, assuming $n_i$ is an integer and $n_i \geq 2$,

$$\begin{aligned} \Delta_i^2 &\geq 2\hat{\sigma}^2 \log T = \frac{2n_i\hat{\sigma}^2 \log T}{n_i} \geq \frac{2\sigma^2\chi^2_{1-\alpha,n_i} \log T}{n_i} \\ &\geq \frac{2\sigma^2\chi^2_{1-\alpha,2} \log T}{n_i} = \frac{-4\sigma^2 \log\alpha \log T}{n_i}. \\ \therefore n_i &\geq \left\lceil \frac{-4\sigma^2 \log\alpha \log T}{\Delta_i^2} \right\rceil = L \geq \frac{-4\sigma^2 \log\alpha \log T}{\Delta_i^2}. \end{aligned}$$

Note that we used the fact that $\chi^2_{1-\alpha,n}$ is monotonically increasing for $n$, therefore $\chi^2_{1-\alpha,n} \geq \chi^2_{1-\alpha,2}$ ($n_i \geq 2$), and that $\chi^2_{1-\alpha,2} = -2\log\alpha$:

$$\begin{aligned} 1 - \alpha &= \chi^2(X < \chi^2_{1-\alpha,n} \mid n = 2) \\ &= \frac{\gamma(\frac{2}{2}, \frac{\chi^2_{1-\alpha,2}}{2})}{\Gamma(\frac{2}{2})} = 1 - e^{-\frac{\chi^2_{1-\alpha,2}}{2}}. \end{aligned}$$

where $\gamma$ and $\Gamma$ are (incomplete) Gamma functions.

10. Using the same union-bound argument used in UCB1,

$$P(\text{LCB}_i(T, n_i) \leq \text{LCB}_*(T, n_*)) \leq 2(T^{-\chi^2_{1-\alpha,n_i}} + 1 - \alpha).$$

11. Assume we followed the UCB1-Normal2 strategy. We use the same argument as UCB1. Assume we pull each arm at least $M$ times in the beginning and $M \leq L$.

$$\begin{aligned} \mathbb{E}[n_i] &\leq L + \sum_{t=K+1}^{T} P(\exists u, v; \text{LCB}_*(t, u) \geq \text{LCB}_i(t, v)) \\ &\leq L + \sum_{t=K+1}^{T} \sum_{u=1}^{t-1} \sum_{v=L}^{t-1} 2(t^{-\frac{3}{8}\chi^2_{1-\alpha,v}} + 1 - \alpha) \\ &\leq L + \sum_{t=K+1}^{T} \sum_{u=1}^{t-1} \sum_{v=L}^{t-1} 2(t^{-\frac{3}{8}\chi^2_{1-\alpha,M}} + 1 - \alpha) \\ &\leq L + \sum_{t=K+1}^{T} \sum_{u=1}^{t} \sum_{v=1}^{t} 2(t^{-\frac{3}{8}\chi^2_{1-\alpha,M}} + 1 - \alpha) \\ &= L + \sum_{t=K+1}^{T} 2(t^{2-\frac{3}{8}\chi^2_{1-\alpha,M}} + (1-\alpha)t^2) \\ &\leq L + 2\sum_{t=1}^{\infty} t^{2-\frac{3}{8}\chi^2_{1-\alpha,M}} + 2(1-\alpha)\sum_{t=1}^{T} t^2 \\ &= L + 2C + 2(1-\alpha)\frac{T(T+1)(2T+1)}{6} \\ &\leq \frac{-4\sigma^2 \log\alpha \log T}{\Delta_i^2} + 1 \quad (\because \lceil x \rceil \leq x + 1) \\ &\quad + 2C + \frac{(1-\alpha)T(T+1)(2T+1)}{3}. \end{aligned}$$

$C$ is a convergent series when

$$2 - \frac{3}{8}\chi^2_{1-\alpha,M} < -1 \Leftrightarrow 8 < \chi^2_{1-\alpha,M}.$$

You can look up the value of $M$ that guarantees this condition from a numerically computed, so-called $\chi^2$-*table* (Table S1). For example, with $\alpha = 0.99$, $8 < \chi^2_{0.01,M}$, thus $M \geq 2$, and with $\alpha = 0.9$, $8 < \chi^2_{0.1,M}$, thus $M \geq 5$. However, the value of $\alpha$ depends on the problem and is unknown prior to solving the problem.

12. Omitted.

| $n$ \ $\alpha$ | 0.995 | 0.99 | 0.975 | 0.95 | 0.90 | 0.10 | 0.05 | 0.025 | 0.01 | 0.005 |
|---|---|---|---|---|---|---|---|---|---|---|
| 1 | — | — | 0.001 | 0.004 | 0.016 | 2.706 | 3.841 | 5.024 | 6.635 | 7.879 |
| 2 | 0.010 | 0.020 | 0.051 | 0.103 | 0.211 | 4.605 | 5.991 | 7.378 | 9.210 | 10.597 |
| 3 | 0.072 | 0.115 | 0.216 | 0.352 | 0.584 | 6.251 | 7.815 | 9.348 | 11.345 | 12.838 |
| 4 | 0.207 | 0.297 | 0.484 | 0.711 | 1.064 | 7.779 | 9.488 | 11.143 | 13.277 | 14.860 |
| 5 | 0.412 | 0.554 | 0.831 | 1.145 | 1.610 | 9.236 | 11.070 | 12.833 | 15.086 | 16.750 |
| 6 | 0.676 | 0.872 | 1.237 | 1.635 | 2.204 | 10.645 | 12.592 | 14.449 | 16.812 | 18.548 |
| 7 | 0.989 | 1.239 | 1.690 | 2.167 | 2.833 | 12.017 | 14.067 | 16.013 | 18.475 | 20.278 |
| 8 | 1.344 | 1.646 | 2.180 | 2.733 | 3.490 | 13.362 | 15.507 | 17.535 | 20.090 | 21.955 |
| 9 | 1.735 | 2.088 | 2.700 | 3.325 | 4.168 | 14.684 | 16.919 | 19.023 | 21.666 | 23.589 |
| 10 | 2.156 | 2.558 | 3.247 | 3.940 | 4.865 | 15.987 | 18.307 | 20.483 | 23.209 | 25.188 |
| 11 | 2.603 | 3.053 | 3.816 | 4.575 | 5.578 | 17.275 | 19.675 | 21.920 | 24.725 | 26.757 |
| 12 | 3.074 | 3.571 | 4.404 | 5.226 | 6.304 | 18.549 | 21.026 | 23.337 | 26.217 | 28.300 |
| 13 | 3.565 | 4.107 | 5.009 | 5.892 | 7.042 | 19.812 | 22.362 | 24.736 | 27.688 | 29.819 |
| 14 | 4.075 | 4.660 | 5.629 | 6.571 | 7.790 | 21.064 | 23.685 | 26.119 | 29.141 | 31.319 |
| 15 | 4.601 | 5.229 | 6.262 | 7.261 | 8.547 | 22.307 | 24.996 | 27.488 | 30.578 | 32.801 |
| 16 | 5.142 | 5.812 | 6.908 | 7.962 | 9.312 | 23.542 | 26.296 | 28.845 | 32.000 | 34.267 |
| 17 | 5.697 | 6.408 | 7.564 | 8.672 | 10.085 | 24.769 | 27.587 | 30.191 | 33.409 | 35.718 |
| 18 | 6.265 | 7.015 | 8.231 | 9.390 | 10.865 | 25.989 | 28.869 | 31.526 | 34.805 | 37.156 |
| 19 | 6.844 | 7.633 | 8.907 | 10.117 | 11.651 | 27.204 | 30.144 | 32.852 | 36.191 | 38.582 |
| 20 | 7.434 | 8.260 | 9.591 | 10.851 | 12.443 | 28.412 | 31.410 | 34.170 | 37.566 | 39.997 |
| 21 | 8.034 | 8.897 | 10.283 | 11.591 | 13.240 | 29.615 | 32.671 | 35.479 | 38.932 | 41.401 |
| 22 | 8.643 | 9.542 | 10.982 | 12.338 | 14.041 | 30.813 | 33.924 | 36.781 | 40.289 | 42.796 |
| 23 | 9.260 | 10.196 | 11.689 | 13.091 | 14.848 | 32.007 | 35.172 | 38.076 | 41.638 | 44.181 |
| 24 | 9.886 | 10.856 | 12.401 | 13.848 | 15.659 | 33.196 | 36.415 | 39.364 | 42.980 | 45.559 |
| 25 | 10.520 | 11.524 | 13.120 | 14.611 | 16.473 | 34.382 | 37.652 | 40.646 | 44.314 | 46.928 |
| 26 | 11.160 | 12.198 | 13.844 | 15.379 | 17.292 | 35.563 | 38.885 | 41.923 | 45.642 | 48.290 |
| 27 | 11.808 | 12.879 | 14.573 | 16.151 | 18.114 | 36.741 | 40.113 | 43.195 | 46.963 | 49.645 |
| 28 | 12.461 | 13.565 | 15.308 | 16.928 | 18.939 | 37.916 | 41.337 | 44.461 | 48.278 | 50.993 |
| 29 | 13.121 | 14.256 | 16.047 | 17.708 | 19.768 | 39.087 | 42.557 | 45.722 | 49.588 | 52.336 |
| 30 | 13.787 | 14.953 | 16.791 | 18.493 | 20.599 | 40.256 | 43.773 | 46.979 | 50.892 | 53.672 |
| 40 | 20.707 | 22.164 | 24.433 | 26.509 | 29.051 | 51.805 | 55.758 | 59.342 | 63.691 | 66.766 |
| 50 | 27.991 | 29.707 | 32.357 | 34.764 | 37.689 | 63.167 | 67.505 | 71.420 | 76.154 | 79.490 |
| 60 | 35.534 | 37.485 | 40.482 | 43.188 | 46.459 | 74.397 | 79.082 | 83.298 | 88.379 | 91.952 |
| 70 | 43.275 | 45.442 | 48.758 | 51.739 | 55.329 | 85.527 | 90.531 | 95.023 | 100.425 | 104.215 |
| 80 | 51.172 | 53.540 | 57.153 | 60.391 | 64.278 | 96.578 | 101.879 | 106.629 | 112.329 | 116.321 |
| 90 | 59.196 | 61.754 | 65.647 | 69.126 | 73.291 | 107.565 | 113.145 | 118.136 | 124.116 | 128.299 |
| 100 | 67.328 | 70.065 | 74.222 | 77.929 | 82.358 | 118.498 | 124.342 | 129.561 | 135.807 | 140.169 |

*Table S1.* $\chi^2_{\alpha,n}$ table.

## S8. The Proof of UCB1-Uniform/Power

Recall the definitions of various LCBs.

$$\begin{array}{lclcll} \text{LCB1}_i & = & \hat{\mu} & - & c & \sqrt{(2\log T)/n_i}. \\ \text{LCB1-Normal}_i & = & \hat{\mu} & - & \hat{\sigma} & \sqrt{(16\log T)/n_i}. \\ \text{LCB1-Normal2}_i & = & \hat{\mu} & - & \hat{\sigma} & \sqrt{2\log T}. \\ \text{LCB1-Uniform}_i & = & \frac{\hat{u}+\hat{l}}{2} & - & (\hat{u}-\hat{l}) & \sqrt{2n_i\log T}. \\ \text{LCB1-Power}_i & = & \frac{\hat{u}\hat{a}}{\hat{a}+1} & - & \hat{u} & \sqrt{2n_i\log T}. \end{array}$$

In the definition of UCB1/UCB1-Normal, the main estimate $\hat{\mu}$ is defined by the sum of i.i.d. random variables for individual rewards, which made it possible to use Hoeffding's inequality in its proof for regret bounds. In contrast, the main estimate $\frac{\hat{u}+\hat{l}}{2}$ and $\frac{\hat{u}\hat{a}}{\hat{a}+1}$ of UCB1-Uniform/Power are not defined from the sum of data points, i.e., $\hat{l} = \min_i x_i$ uses a minimum, $\hat{u} = \max_i x_i$ uses a maximum, and $\hat{a} = \left(\log \hat{u} - \frac{1}{N}\sum_i \log x_i\right)^{-1}$ uses both a maximum and a logarithmic sum. To handle these cases, we need concentration inequalities for more general functions other than sums. Among many concentration inequalities for general functions (e.g., Efron-Stein inequality, Han's inequality, logarithmic Sobolev inequality (Boucheron et al., 2013)), we found that *bounded differences inequality* (Boucheron et al., 2013) can be used as the basis of the proof of UCB1-Power and UCB1-Uniform.

### S8.1. Preliminary: Bounded Difference Inequality

To use the inequality, we must assume a function with bounded differences, so let's define it first.

**Definition 4** (Functions with Bounded Differences). *A $n$-ary function $g : X^n \to \mathbb{R}$ for a set $X$ has a* bounded difference *when, for all $1 \le i \le n$, there exists a constant $c_i \in \mathbb{R}$ such that*

$$\max_{y\in X}\left|\begin{array}{l} g(\ldots, x_{i-1}, x_i, x_{i+1}, \ldots) \\ -g(\ldots, x_{i-1}, y, x_{i+1}, \ldots) \end{array}\right| < c_i.$$

Note that an MLE of a parameter obtained from $n$ sample points $(x_1, \ldots, x_n)$ are $n$-ary function. Moreover, quantities defined from the parameters obtained by MLE are also one of them. For example, the MLE is $u$ in $U(l, u)$ is $\hat{u} = \max_i x_i$, which is a function of $(x_1, \ldots, x_n)$, and the mean $\frac{\hat{l}+\hat{u}}{2}$ of the fitted distribution $U(\hat{l}, \hat{u})$ is also a function of $(x_1, \ldots, x_n)$.

When the distribution function of a random variable has bounded differences, then we can bound its tail probability as follows. This inequality generalizes Hoeffding's inequality by $g(\mathrm{x}_1, \ldots, \mathrm{x}_n) = \sum_{i=1}^n \mathrm{x}_i$.

**Theorem 6** (Bounded Differences Inequality). *When a $n$-ary function $g : X^n \to \mathbb{R}$ for a set $X$ has a bounded difference $c_1, \ldots c_n$ for each argument, let $C = \sum_{i=1}^n c_i^2$. Then a random variable $\mathrm{z}_n = g(\mathrm{x}_1, \ldots, \mathrm{x}_n)$ satisfies*

$$P(|\mathrm{z}_n - \mathbb{E}[\mathrm{z}_n]| \ge \delta) \le \exp -2\delta^2/C.$$

**Theorem 7** (Hoeffding's Inequality). *Given random variables $\mathrm{x}_i \in [a, b]$, let their sum be $\mathrm{S}_n = \sum_{i=1}^n \mathrm{x}_i$ and $C = \sum_{i=1}^n |b_i - a_i|^2$. Then $\mathrm{S}_n$ satisfies*

$$P(|\mathrm{S}_n - \mathbb{E}[\mathrm{S}_n]| \ge \delta) \le \exp -2\delta^2/C.$$

Due to the similarity of the form, once we show that the quantities used in LCB-Uniform/Power have bounded difference, it is straightforward to prove their regret.

### S8.2. Preliminary: Order Statistics

The proof of UCB1-Uniform relies on several theorems in order statistics ().

**Definition 5** (Order Variable). *Assume $n$ random variables $\mathrm{x}_1, \ldots \mathrm{x}_n$. Let $\mathrm{x}_{(k)}$ denote a $k$-th* order variable *defined as*

$$\mathrm{x}_{(k)} = \textit{the } k\textit{-th largest of } \mathrm{x}_1, \ldots \mathrm{x}_n.$$

*In other words, $\mathrm{x}_{(1)} \le \mathrm{x}_{(2)} \le \ldots \le \mathrm{x}_{(n)}$, where $\mathrm{x}_{(1)}$ is the smallest and $\mathrm{x}_{(k)}$ is the largest.*

**Definition 6** (Range Variable). *Given order variables $\mathrm{x}_{(1)}, \ldots \mathrm{x}_{(n)}$, a* range variable *is $\mathrm{R}_n = \mathrm{x}_{(n)} - \mathrm{x}_{(1)}$.*

**Lemma 1** (CDF of range variable ()). *Assume $n$ i.i.d. random variables $\mathrm{x}_1, \ldots \mathrm{x}_n$ with a CDF $F$ and a PDF $f$. The cumulative distribution function of $\mathrm{R}_n$ is given by*

$$P(\mathrm{R}_n < r) = n\int (F(x+r) - F(x))^{n-1} f(x)dx.$$

### S8.3. The Proof of UCB1-Uniform

To prove the regret bound for UCB1-Uniform, we first prove two lemmas.

**Lemma 2** (CDF of range variable for $U(0,1)$). *Assume $n$ i.i.d. random variables $\mathrm{x}_1, \ldots \mathrm{x}_n \sim U(0,1)$. The cumulative distribution function of $\mathrm{R}_n$ is $P(\mathrm{R}_n < r) = nr^{n-1}$.*

*Proof.* $P(\mathrm{R}_n < r)$

$$= n\int_0^1 ((x+r) - x)^{n-1} \cdot 1 \cdot dx$$

$$= n\int_0^1 r^{n-1}dx = n\left[r^{n-1}x\right]_0^1 = nr^{n-1}(1-0) = nr^{n-1}.$$

□

**Lemma 3.** *Assume i.i.d. RVs $\mathrm{x}_1, \ldots \mathrm{x}_n \sim U(l, u)$, $\mathrm{x}_{(1)} = \hat{l}$ and $\mathrm{x}_{(n)} = \hat{u}$. Then $\mathrm{z}_n = g(\mathrm{x}_1, \mathrm{x}_2, \ldots, \mathrm{x}_n) = \frac{\hat{u}+\hat{l}}{2} = \frac{\mathrm{x}_{(n)}+\mathrm{x}_{(1)}}{2}$ has a bounded difference $u - l$.*

*Proof.* First, $g(\mathrm{x}_1, \dots \mathrm{x}_i, \dots \mathrm{x}_n) \in [l, u]$ because

$$l = \frac{l+l}{2} < \frac{\mathrm{x}_{(n)} + \mathrm{x}_{(1)}}{2} < \frac{u+u}{2} = u.$$

The same trivially holds for $g(\mathrm{x}_1, \dots y, \dots \mathrm{x}_n) \in [l, u]$ when $y \in [l, u]$. Their difference is largest when either one is $u$ and another one is $l$. Thus

$$\left| \; g(\dots, \mathrm{x}_i, \dots) - g(\dots, y, \dots) \; \right| < u - l.$$

□

This results in $C = \sum_i c_i^2 = n(u-l)^2$, therefore

$$P(A : |\mathrm{z}_n - \mathbb{E}\mathrm{z}_n| \geq \delta) \leq \exp -\frac{2\delta^2}{n(u-l)^2}.$$

Now we prove the upper bound of the cumulative regret of the LCB1-Uniform parameterized by $g$, LCB1-Uniform$_i(g) = \frac{\hat{u}_i + \hat{l}_i}{2} - (\hat{u}_i - \hat{l}_i)\sqrt{g n_i \log T}$, where $\hat{u}_i, \hat{l}_i$ are the empirical max/min of samples from arm $i$, $n_i$ is the number of pulls from arm $i$, and $T = \sum_{i=1}^{K} n_i$ is the total pulls from all $K$ arms. Later, the best $g$ is determined to be $g = 6$.

1. As shown above.

2. Same as UCB1.

3. Same as UCB1.

4. Same as UCB1.

5. Let $\delta = (\hat{u}_i - \hat{l}_i)\sqrt{g n_i \log T}$. and $r_i = \frac{\hat{u}_i - \hat{l}_i}{u_i - l_i} \in [0, 1]$. Then

$$\begin{aligned} P(A) &\leq \exp -\frac{2(\hat{u}_i - \hat{l}_i)^2 \cdot g n_i \log T}{n_i (u_i - l_i)^2} \\ &= \exp -2 g r_i^2 \log T = T^{-2 g r_i^2}. \end{aligned}$$

   The trick starts here. The value of $r_i = \frac{\hat{u}_i - \hat{l}_i}{u_i - l_i}$ is unavailable because we do not know the true bounds $u_i$ and $l_i$. However, if event $B : r_i \geq X$ holds for some constant $X$, we would obtain a more convenient form $T^{-2gX^2}$:

$$P(A) \leq T^{-2 g r_i^2} \leq T^{-2gX^2}.$$

   Assume $P(B) = \alpha$. Note that $r_i = \frac{\hat{u}_i - \hat{l}_i}{u_i - l_i}$ is a range variable for $n_i$ i.i.d. RVs from $U(0, 1)$. Therefore, from its CDF, for some $X \in [0, 1]$,

$$P(r_i < X) = n X^{n-1}.$$

   Solving $X$ for $P(r_i < X) = P(\neg B) = 1 - \alpha$, we obtain

$$X_{n, 1-\alpha} = \left( \frac{1-\alpha}{n} \right)^{\frac{1}{n-1}}.$$

   $A$ and $B$ could be correlated. Using union-bound

$$\begin{aligned} P(\neg(A \wedge B)) &= P(\neg A \vee \neg B) \leq P(\neg A) + P(\neg B) \\ 1 - P(A \wedge B) &\leq 1 - P(A) + P(\neg B) \\ \therefore P(A) &\leq P(A \wedge B) + P(\neg B) \\ &= T^{-2gX_{n,1-\alpha}^2} + 1 - \alpha. \end{aligned}$$

6. From $2\delta \leq \Delta_i$ and using the fact that $n_i$ is an integer,

$$\begin{aligned} & \Delta_i \geq 2(\hat{u}_i - \hat{l}_i)\sqrt{g n_i \log T} \\ \Leftrightarrow \; & \Delta_i^2 \geq 4g(\hat{u}_i - \hat{l}_i)^2 n_i \log T \\ & = 4g(u_i - l_i)^2 r_i^2 n_i \log T \\ & \geq 4g(u_i - l_i)^2 X_{n_i, 1-\alpha}^2 n_i \log T \\ & = 4g(u_i - l_i)^2 \left( \frac{1-\alpha}{n_i} \right)^{\frac{2}{n_i - 1}} n_i \log T \\ & \geq 4g(u_i - l_i)^2 \left( \frac{1-\alpha}{n_i} \right)^2 n_i \log T \\ & \left( \because 0 < \frac{1-\alpha}{n_i} < 1, \; \frac{2}{n_i - 1} < 2 \right) \\ \Leftrightarrow \; & n_i \geq \frac{4g(u_i - l_i)^2 (1-\alpha)^2 \log T}{\Delta_i^2} \\ \therefore \; & n_i \geq L = \left\lceil \frac{4g(u_i - l_i)^2 (1-\alpha)^2 \log T}{\Delta_i^2} \right\rceil \end{aligned}$$

7. Using the same union-bound argument as UCB1,

$$P(\mathrm{LCB}_i(T, n_i) \leq \mathrm{LCB}_*(T, n_*)) \leq 2T^{-2gX_{n_i,1-\alpha}} + 2 - 2\alpha.$$

8. For a reason explained later, we require each arm to be pulled at least $M$ times. For a fixed $\alpha$, the solution $X_{n_i, 1-\alpha}$ of $X$ for $P(r_i < X) = 1 - \alpha$ increases monotonically as $n_i$ increases. Therefore, $X_{n_i, 1-\alpha} \geq X_{M, 1-\alpha}$ under $n_i \geq M$. Then, using the same argument as UCB1,

$$\begin{aligned} \mathbb{E}[n_i] &\leq L + \sum_{t=1}^{T} t^2 (2t^{-2gX_{M,1-\alpha}} + 2(1-\alpha)) \\ &\leq L + 2\sum_{t=1}^{\infty} t^{2-2gX_{M,1-\alpha}} + 2(1-\alpha)\sum_{t=1}^{T} t^2 \\ &\leq L + 2C + \frac{(1-\alpha)T(T+1)(2T+1)}{3} \\ &\leq \frac{8(u_i - l_i)^2 (1-\alpha)^2 \log T}{\Delta_i^2} + 1 \\ &\quad + 2C + \frac{(1-\alpha)T(T+1)(2T+1)}{3} \end{aligned}$$

$(\because \lceil x \rceil \leq x+1)$

We introduced $M$ because $C$ is convergent only when the exponentiator of $t$ is below $-1$. We consider the condition in which an integer $M$ exists for a given $\alpha$. Consider:

$$2 - 2gX_{x,1-\alpha} = 2 - 2g\left(\frac{1-\alpha}{x}\right)^{\frac{2}{x-1}} < -1$$
$$\Leftrightarrow f(x) = x^2\left(\frac{3}{2g}\right)^{x-1} < (1-\alpha)^2$$

Since $1-\alpha \in [0,1]$, this is satisfiable only when $0 \leq f(x) \leq 1$. Positivity is trivial. To satisfy $\forall x \geq M; f(x) \leq 1$, it is sufficient if $f(M) \leq 1$ and $\forall x \geq M; f'(x) < 0$. From the derivative below,

$$f'(x) = x\left(\frac{3}{2g}\right)^{x-1}\left(2 + x\log\frac{3}{2g}\right),$$

this condition is achieved when $3/2g < 1$. If $g = 2$, then $f(22) > 1 > f(23)$, thus it requires too many initialization pulls: $M = 23$. For MCTS where we evaluate each node at least once, we wish to achieve $M = 2$. $g = 6$ achieves $f(2) = 1$, thus is the ideal parameter for MCTS.

9. The regret is polynomial.

$$Tz_* - \sum_{i=1}^{K} z_i \mathbb{E}[n_i] = \sum_{i=1}^{K}(z_* - z_i)\mathbb{E}[n_i] = \sum_{i=1}^{K}\Delta_i \mathbb{E}[n_i]$$
$$\leq \sum_{i=1}^{K}\Delta_i \left(\begin{array}{c} \frac{4g(u_i-l_i)^2(1-\alpha)^2\log T}{\Delta_i^2} + 1 + 2C \\ + \frac{(1-\alpha)T(T+1)(2T+1)}{3} \end{array}\right).$$

### S8.4. The Proof of UCB1-Power

To prove the regret bound for UCB1-Uniform, we prove three lemmas.

**Lemma 4** (CDF of range variable for $\mathrm{Pow}(a,1)$)**.** *Assume $n$ i.i.d. random variables $\mathrm{x}_1, \dots \mathrm{x}_n \sim \mathrm{Pow}(a,1)$. The cumulative distribution function of $\mathrm{R}_n$ is not analytical.*

*Proof.* $P(\mathrm{R}_n < r)$

$$= n\int_0^1 ((x+r)^a - x^a)^{n-1} a x^{a-1} dx$$
$$= -\int_0^1 anx^{an-1}dx + an\int_0^1 (x+r)^{a(n-1)}x^{a-1}dx$$

The first term is

$$\int_0^1 anx^{an-1}dx = [x^{an}]_0^1 = 1$$

For the second term, let $b = a(n-1)$ and $c = a-1$. If $b$ was an integer, the taylor expansion of $(x+r)^b$ yields

$$\int_0^1 (x+r)^b x^c dx = \int_0^1 \sum_{k=0}^{\infty} \binom{b}{k} r^{b-k} x^k x^c dx$$

where $\binom{b}{k} = \frac{b!}{k!(b-k)!}$. Since $b$ is real, we can generalize it with Gamma function as $\binom{b}{k} = \frac{\Gamma(b+1)}{\Gamma(k+1)\Gamma(b-k+1)}$, but this has little to do with the later derivation. Continuing,

$$= \int_0^1 \sum_{k=0}^{\infty} \binom{b}{k} r^{b-k} x^{c+k} dx = \sum_{k=0}^{\infty} \binom{b}{k} r^{b-k} \int_0^1 x^{c+k} dx$$
$$= \sum_{k=0}^{\infty} \binom{b}{k} r^{b-k} \left[\frac{x^{c+k+1}}{c+k+1}\right]_0^1 = \sum_{k=0}^{\infty} \binom{b}{k} r^{b-k} \frac{1}{c+k+1}.$$

Thus we obtain a non-analytical form,

$$P(\mathrm{R}_n < r) = -1 + \sum_{k=0}^{\infty} \binom{a(n-1)}{k} r^{a(n-1)-k} \frac{1}{a+k}.$$

□

Although the CDF of $\mathrm{R}_n$ is not analytical, we can bound it from above.

**Lemma 5** (CDF of range variable for $\mathrm{Pow}(a,1)$)**.** *Assume $n$ i.i.d. random variables $\mathrm{x}_1, \dots \mathrm{x}_n \sim \mathrm{Pow}(a,1)$. The cumulative distribution function of $\mathrm{R}_n$ can be bounded from above as $P(\mathrm{R}_n < r) \le (1+r)^{an} - r^{an} - 1$.*

*Proof.* To bound this CDF from above,

$$P(\mathrm{R}_n < r) = -1 + an\int_0^1 (x+r)^{a(n-1)}x^{a-1}dx$$
$$\le -1 + an\int_0^1 (x+r)^{a(n-1)}(x+r)^{a-1}dx$$
$$= -1 + an\int_0^1 (x+r)^{an-1}dx$$
$$= -1 + [(x+r)^{an}]_0^1$$
$$= -1 + (1+r)^{an} - r^{an}.$$

□

**Lemma 6** (Critical value of range variable for $\mathrm{Pow}(a,1)$)**.** *Assume $n$ i.i.d. random variables $\mathrm{x}_1, \dots \mathrm{x}_n \sim \mathrm{Pow}(a,1)$. The critical value $r$ for $P(\mathrm{R}_n < r) = 1-\alpha$ is bounded by:*

$$(2^{an} + \alpha - 2)^{1/an} \ge r \ge \frac{(3-\beta)(\beta-1)}{2n}$$

*with $\beta = (2-\alpha)^{1/a}$.*

*Proof.* The upper-bound is shown as follows:

$$1-\alpha \le (1+r)^{an} - r^{an} - 1.$$
$$2-\alpha \le (1+r)^{an} - r^{an}$$
$$r^{an} \le (1+r)^{an} + \alpha - 2$$
$$\le 2^{an} + \alpha - 2$$
$$r \le (2^{an} + \alpha - 2)^{1/an}.$$

The lower-bound is shown as follows:

$$1-\alpha \le (1+r)^{an} - r^{an} - 1.$$
$$2-\alpha \le (1+r)^{an} - r^{an}$$
$$\le (1+r)^{an}.$$
$$(2-\alpha)^{1/an} \le 1+r.$$
$$r \ge (2-\alpha)^{1/an} - 1.$$

Since $1-\alpha \in [0,1]$, $2-\alpha \in [1,2]$, therefore $(2-\alpha)^{1/a} \in [1, 2^{1/a}]$. Let $\beta = (2-\alpha)^{1/a}$. From the Taylor expansion,

$$x^{1/n} = 1 + \frac{x-1}{n} - \frac{(n-1)(x-1)^2}{2n^2} + \frac{(n-1)(2n-1)(x-1)^3}{3n^3} \dots$$
$$= 1 + \sum_{k=1}^{\infty} (-1)^k \frac{\left(\prod_{j=1}^{k-1}(jn-1)\right)(x-1)^k}{kn^k}$$
$$\ge 1 + \frac{x-1}{n} - \frac{(n-1)(x-1)^2}{2n^2}.$$

Using this,

$$r \ge 1 + \frac{\beta-1}{n} - \frac{(n-1)(\beta-1)^2}{2n^2} - 1$$
$$= \frac{\beta-1}{n} - \frac{(n-1)(\beta-1)^2}{2n^2}$$
$$= \frac{\beta-1}{n} - \frac{(\beta-1)^2}{2n} + \frac{(\beta-1)^2}{2n^2}$$

$$\geq \frac{\beta - 1}{n} - \frac{(\beta - 1)^2}{2n} = \frac{(3-\beta)(\beta - 1)}{2n}.$$

□

**Lemma 7.** *Assume i.i.d. RVs* $\mathrm{x}_1, \ldots \mathrm{x}_n \sim \mathrm{Pow}(a, u)$*,* $\mathrm{x}_{(n)} = \hat{u}$ *and* $\hat{a} = \left(\log \hat{u} - \frac{1}{n}\sum_i \log x_i\right)^{-1}$*. Then* $\mathrm{z}_n = g(\mathrm{x}_1, \mathrm{x}_2, \ldots, \mathrm{x}_n) = \frac{\hat{u}\hat{a}}{\hat{a}+1}$ *has a bounded difference* $u$*.*

*Proof.* First, note that $\hat{a} > 0$ because

$$\log \hat{u} - \frac{1}{n}\sum_i \log x_i = \frac{1}{n}\sum_i \log \frac{\hat{u}}{x_i} > 0.$$

Therefore

$$0 \leq \mathrm{z}_n = \frac{\hat{u}\hat{a}}{\hat{a}+1} = \frac{\hat{u}}{1 + \hat{a}^{-1}} \leq \hat{u} \leq u.$$

If we compute the bounded difference, both $g(\mathrm{x}_1, \ldots \mathrm{x}_i, \ldots \mathrm{x}_n)$ and $g(\mathrm{x}_1, \ldots y, \ldots \mathrm{x}_n)$ are in $[0, u]$, assuming $y \in [0, u]$. Therefore, trivially

$$\left| \; g(\ldots, \mathrm{x}_i, \ldots) - g(\ldots, y, \ldots) \; \right| < u.$$

□

This results in $C = \sum_i c_i^2 = nu^2$, therefore

$$P(A : |\mathrm{z}_n - \mathbb{E}\mathrm{z}_n| \geq \delta) \leq \exp - \frac{2\delta^2}{nu^2}.$$

Now we prove the upper bound of the cumulative regret of LCB1-Power$_i = \frac{\hat{u}_i\hat{a}_i}{\hat{a}_i+1} - \hat{u}_i\sqrt{2n_i \log T}$.

1. As shown above.
2. Same as UCB1.
3. Same as UCB1.
4. Same as UCB1.
5. Let $\delta = \hat{u}_i\sqrt{2n_i \log T}$ and $r_i = \frac{\hat{u}_i}{u_i} \in [0, 1]$. Then

$$\begin{aligned} P(A) &\leq \exp - \frac{2\hat{u}_i^2 \cdot 2n_i \log T}{n_i u^2} \\ &= \exp -4r_i^2 \log T = T^{-4r_i^2}. \end{aligned}$$

   The trick starts here. The value of $r_i = \frac{\hat{u}_i}{u_i}$ is unavailable because we do not know the true bound $u_i$. However, if event $B : r_i \geq X$ holds for some constant $X$, we would obtain a more convenient form $T^{-4X^2}$:

$$P(A) \leq T^{-4r_i^2} \leq T^{-4X^2}.$$

   Assume $P(B) = \alpha$. Note that $r_i = \frac{\hat{u}_i}{u_i}$ is a range variable for $n_i$ i.i.d. RVs from $\mathrm{Pow}(a, 1)$. Therefore, let $X_{n_i,1-\alpha}$ be the critical value of the range variable CDF at $P(r_i < X) = 1 - \alpha$, even though it is not analytically available. $A$ and $B$ could be correlated. Using union-bound

$$\begin{aligned} P(\neg(A \wedge B)) &= P(\neg A \vee \neg B) \leq P(\neg A) + P(\neg B) \\ 1 - P(A \wedge B) &\leq 1 - P(A) + P(\neg B) \\ \therefore P(A) &\leq P(A \wedge B) + P(\neg B) \\ &= T^{-4X^2_{n_i,1-\alpha}} + 1 - \alpha. \end{aligned}$$

6. From $2\delta \leq \Delta_i$ and using the fact that $n_i$ is an integer,

$$\begin{aligned} \Delta_i &\geq 2\hat{u}_i\sqrt{2n_i \log T} \\ \Leftrightarrow \Delta_i^2 &\geq 8\hat{u}_i^2 n_i \log T \\ &= 8u_i^2 r_i^2 n_i \log T \\ &\geq 8u_i^2 X^2_{n_i,1-\alpha} n_i \log T \\ &\geq 8u_i^2 \left(\frac{(3-\beta)(\beta-1)}{2n_i}\right)^2 n_i \log T \\ &= 2u_i^2 (3-\beta)^2(\beta-1)^2 \frac{\log T}{n_i} \\ &\quad (\because \text{Lemma. 6, lower bound}) \\ \Leftrightarrow n_i &\geq \frac{2u_i^2(3-\beta)^2(\beta-1)^2 \log T}{\Delta_i^2} \\ \therefore n_i &\geq L = \left\lceil \frac{2u_i^2(3-\beta)^2(\beta-1)^2 \log T}{\Delta_i^2} \right\rceil \end{aligned}$$

   Here, $\beta = (2 - \alpha)^{1/a}$.

7. Using the same union-bound argument as UCB1,

$$P(\mathrm{LCB}_i(T, n_i) \leq \mathrm{LCB}_*(T, n_*)) \leq 2T^{-4X_{n_i,1-\alpha}} + 2 - 2\alpha.$$

8. For a reason explained later, we require each arm to be pulled at least $M$ times. For a fixed $\alpha$, the solution $X_{n_i,1-\alpha}$ of $X$ for $P(r_i < X) = 1 - \alpha$ increases monotonically as $n$ increases. Therefore, $X_{n_i,1-\alpha} \geq X_{M,1-\alpha}$ under $n_i \geq M$.

   Then, using the same argument as UCB1,

$$\begin{aligned} \mathbb{E}[n_i] &\leq L + \sum_{t=1}^{T} t^2(2t^{-4X_{M,1-\alpha}} + 2(1-\alpha)) \\ &\leq L + 2\sum_{t=1}^{\infty} t^{2-4X_{M,1-\alpha}} + 2(1-\alpha)\sum_{t=1}^{T} t^2 \\ &\leq L + 2C + \frac{(1-\alpha)T(T+1)(2T+1)}{3} \\ &\leq \frac{2u^2(3-\beta)^2(\beta-1)^2 \log T}{\Delta_i^2} + 1 \end{aligned}$$

$$+ 2C + \frac{(1-\alpha)T(T+1)(2T+1)}{3}$$
$$(\because \lceil x \rceil \leq x+1)$$

We introduced $M$ because $C$ is convergent only when the exponentiator of $t$ is below $-1$. We consider the condition in which an integer $M$ exists for a given $\alpha$. Consider:

$$2 - 4X_{x,1-\alpha} < -1 \Leftrightarrow \frac{3}{4} < X_{x,1-\alpha}.$$

If some $x$ satisfies this inequality, then it must hold

$$\frac{3}{4} < X_{x,1-\alpha} < (2^{ax} + \alpha - 2)^{1/ax}$$
$$(\because \text{Lemma. 6, upper bound})$$
$$\Leftrightarrow \left(\frac{3}{4}\right)^{ax} - 2^{ax} + 2 = f(x) < \alpha$$

$f(x)$ is monotonically decreasing. Then $M$ is the smallest integer that satisfies this formula, i.e., $M = \inf\{x \in \mathbb{Z} | f(x) < \alpha\}$. For example, when $a = \frac{1}{2}$ and $\alpha = \frac{1}{2}$, the solution to $f(x) = \alpha$ is between 2 and 3 ($f(2) = 0.75 > \alpha = 0.5 > f(3) > -0.18$), therefore $M = 3$. $M$ depends on unknown $a$ and $\alpha$, thus we simply assume $M = 1$ works (evaluating each node once).

9. The regret is polynomial.

$$Tz_* - \sum_{i=1}^{K} z_i \mathbb{E}[n_i] = \sum_{i=1}^{K} (z_* - z_i)\mathbb{E}[n_i] = \sum_{i=1}^{K} \Delta_i \mathbb{E}[n_i]$$
$$\leq \sum_{i=1}^{K} \Delta_i \left( \begin{array}{l} \frac{2u^2(3-\beta)^2(\beta-1)^2 \log T}{\Delta_i^2} + 1 + 2C \\ + \frac{(1-\alpha)T(T+1)(2T+1)}{3} \end{array} \right).$$

# S9. Full Results

## S9.1. Cumulative Histograms for All Heuristics and All Search Statistics

Fig. S1-S3 shows the cumulative histogram of the number of instances solved by a particular evaluation/expansion/runtime.

# References


Auer, P., Cesa-Bianchi, N., and Fischer, P. Finite-Time Analysis of the Multiarmed Bandit Problem. *Machine Learning*, 47(2-3):235–256, 2002.

Bonet, B. and Geffner, H. Planning as Heuristic Search. *Artificial Intelligence*, 129(1):5–33, 2001.

Boucheron, S., Lugosi, G., and Massart, P. *Concentration Inequalities: A Nonasymptotic Theory of Independence*. Oxford University Press, 2013.

Bylander, T. A Probabilistic Analysis of Prepositional STRIPS Planning. *Artificial Intelligence*, 81(1):241–271, 1996.

Fikes, R. E., Hart, P. E., and Nilsson, N. J. Learning and Executing Generalized Robot Plans. *Artificial Intelligence*, 3 (1-3):251–288, 1972. doi: 10.1016/0004-3702(72)90051-3.

Hoffmann, J. and Nebel, B. The FF Planning System: Fast Plan Generation through Heuristic Search. *J. Artif. Intell. Res.(JAIR)*, 14:253–302, 2001. doi: 10.1613/jair.855.

Richter, S., Thayer, J. T., and Ruml, W. The Joy of Forgetting: Faster Anytime Search via Restarting. In *Proc. of ICAPS*, 2010.

Richter, S., Westphal, M., and Helmert, M. LAMA 2008 and 2011. In *Proc. of IPC*, pp. 117–124, 2011.

Schulte, T. and Keller, T. Balancing Exploration and Exploitation in Classical Planning. In *Proc. of SOCS*, 2014.

Vershynin, R. *High-Dimensional Probability: An Introduction with Applications in Data Science*. Cambridge Series in Statistical and Probabilistic Mathematics. Cambridge University Press, 2018. doi: 10.1017/9781108231596.

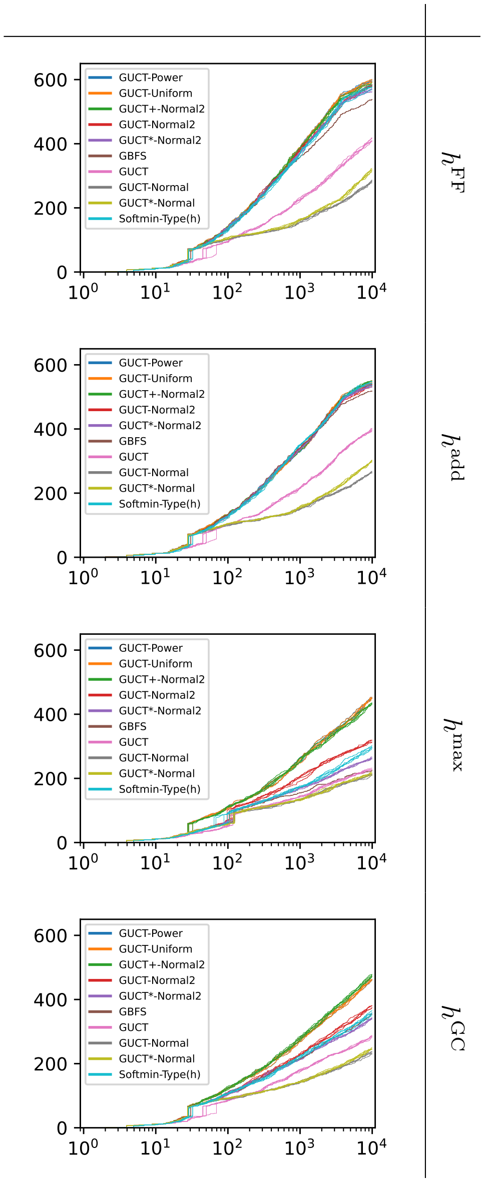


*Figure S1.* The cumulative histogram of the number of problem instances solved ($y$-axis) below a certain number of node evaluations ($x$-axis, 10,000 nodes maximum). Each line represents a random seed. The total numbers at the limit differ from those in other plots (this result does not limit the expansions or the runtime).

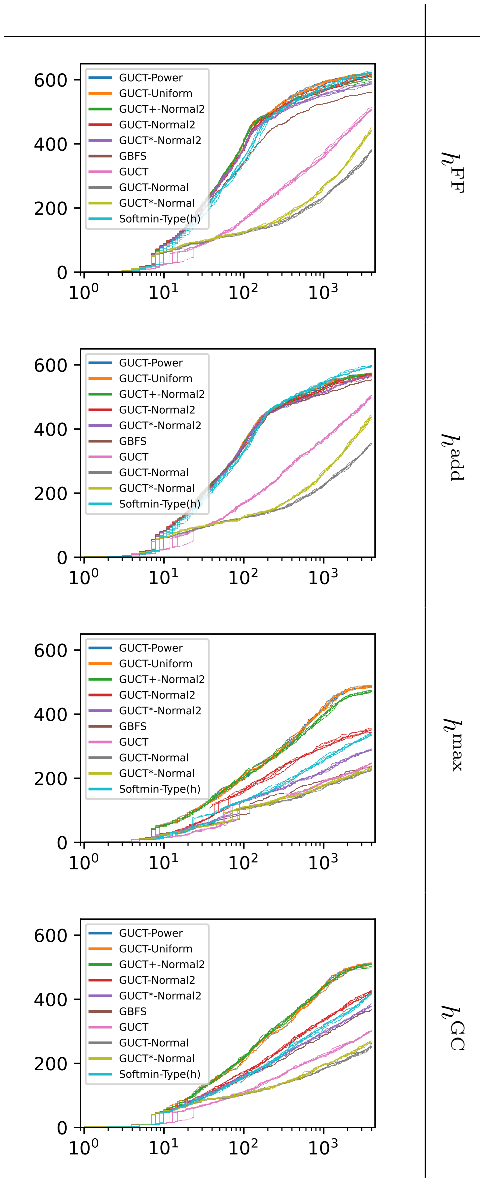


*Figure S2.* The cumulative histogram of the number of problem instances solved ($y$-axis) below a certain number of node expansions ($x$-axis, 4,000 nodes maximum). Each line represents a random seed. The total numbers at the limit differ from those in other plots (this result does not limit the evaluations or the runtime).

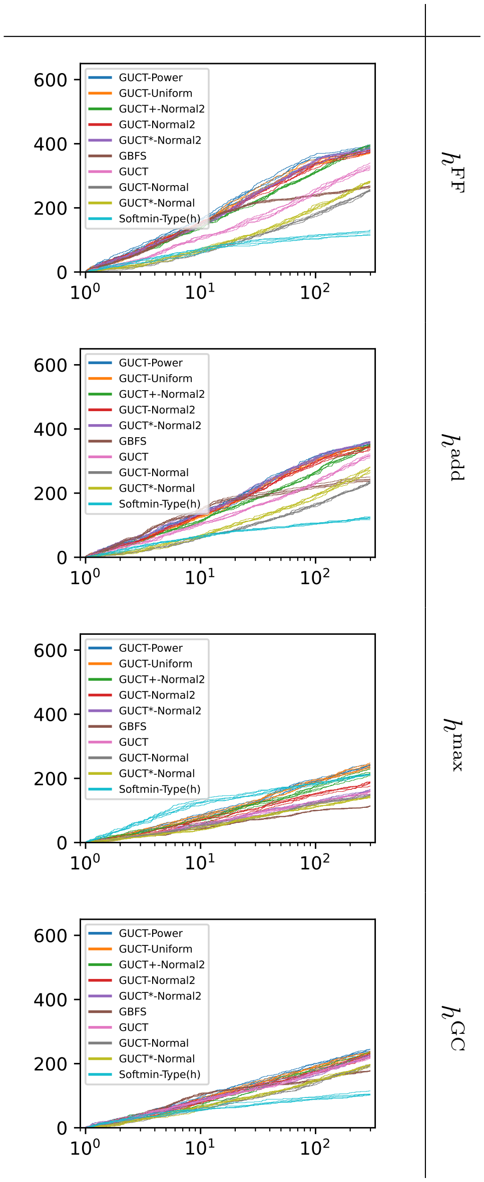


*Figure S3.* The cumulative histogram of the number of problem instances solved ($y$-axis) below a certain runtime ($x$-axis, 300 seconds maximum). Each line represents a random seed. The total numbers at the limit differ from those in other plots (this result does not limit the evaluations or the expansion).
